# Supplementary material for: Added costs of insect-scale flapping flight in unsteady airflows
Source: arXiv:1610.09101 source file (2016-10-28)
Supplement: Supplementary file 1 [file supplementary_material.pdf]

# Added costs of insect-scale flapping flight in unsteady airflows.

# Supplementary material

Dmitry Kolomenskiy[1,*], Sridhar Ravi[2,3,*], Taku Takabayashi[1], Teruaki Ikeda[1], Kohei Ueyama[1], Thomas Engels[4], Alex Fisher[2], Hiroto Tanaka[5], Kai Schneider[6], Jörn Sesterhenn[4] and Hao Liu[1,7]

[1]Graduate School of Engineering, Chiba University, Chiba, Japan
[2]School of Aerospace Mechanical and Manufacturing Engineering, RMIT University, Melbourne, Australia
[3]Department of Neurobiology, University of Bielefeld, Bielefeld, Germany
[4]ISTA, Technische Universität Berlin, Berlin, Germany
[5]Department of Mechanical Engineering, School of Engineering, Tokyo Institute of Technology, Tokyo, Japan
[6]I2M - UMR 7373 - CNRS, Centre de Mathématiques et d'Informatique, Aix-Marseille Université, Marseille, France
[7]Shanghai-Jiao Tong University and Chiba University International Cooperative Research Centre (SJTU-CU ICRC), Shanghai, China
[*]Equal contributions

October 3, 2016

## S1 Robotic flapper

In this study we use the hummingbird-inspired robotic flapper developed in earlier work [8, 4]. The rotational speed of an electric DC motor is geared down by 8 times using a planetary gear mechanism. Then, the rotational output is converted to reciprocating flapping motion using a slider and a seesaw mechanism. Two bilateral wings

are attached at the flapper. The stroke amplitude of the flapping motion is set to 110 degrees. Constant voltage ranging from 2.5 to 3.5 V is applied to the DC motor using a stabilized power supply. During the tests, the voltage and current drawn by the flapper were measured using a DL850E ScopeCorder (Yokogawa Meters & Instruments Corp., Japan) data logger.

All components of the flapper are made from Polyether Ether Fetone (PEEK) and Acrylonitrile Butadiene Styrene (ABS) copolymer on a micro-mill. The wings consist of polyimide film (Kapton) with carbon fibre reinforced leading edge and wing root. The wing planform is semi-elliptical (see figure 2$b$) and it is inspired by hummingbird wings. Prior measurements showed that this wing planform produced high lift and the wings were durable over many flapping cycles, see [9]. The leading edge is rigidly attached to the wing root hence all feathering undergone by the wings is passive mainly due to the deformation of the Kapton membrane.

In the 2-DOF experiments, the lift (vertical force) produced by the flapping wings at maximum safe power was lower than the combined mass of the flapper and rail fixtures (7 g). A helium balloon that provided 3 gf of lift was tied to the flapper to counteract the added mass of the fixture and facilitate motion. The balloon was placed outside the wind tunnel and attached to the flapper using a minimal friction string through a porthole, see figure 2($e$). The balloon would possibly affect the time resolved dynamics of the vertical motion of the flapper. However, it cannot affect the mean displacement of the flapper which is the quantity of interest in this study.

# S2 Numerical model of a bumblebee

We use an open source software FluSI [3]. It is an incompressible Navier–Stokes solver based on a Fourier pseudo-spectral method with volume penalization. It is designed for direct numerical simulation (DNS) of turbulent flows, i.e., the numerical discretization resolves all turbulent scales without any turbulence modelling being involved. The bumblebee model considered here has the morphological and kinematical parameters as described in [2]. The insect is approximated by the body and two rigid wings, which move with respect to each other. The wing length is equal to $R = 13.2$ mm, the wingbeat frequency is $f = 152$ Hz.

To generate an unsteady inflow, a vertical cylinder with diameter $D = 25$ mm is placed near the inflow boundary, as shown in the flow visualization in figure 5($a$). The inflow velocity is equal to $U_\infty = 2.5$ m/s. To reduce the computational cost, the Reynolds number based on the wing parameters is set to $Re = 470$ (i.e., $Re_D = 1000$ based on $D$ and $U_\infty$) by increasing the kinematic viscosity by a factor of 4 compared to the experimental conditions. The aerodynamic force coefficients depend on the Reynolds number as $\mathcal{O}(Re^0)$ in the range of $Re$ considered in this study, therefore, lower-Reynolds number computations can provide conclusive estimates.

The flow domain is discretized using a uniform Cartesian grid consisting of 283 million points ($960 \times 768 \times 384$ in the longitudinal, lateral and vertical directions, respectively). The volume penalization parameter is equal to $C_\eta = 2.5 \cdot 10^{-4}$.

In the 1-DOF numerical simulation, the axis of rotation passed through the body center of mass. The roll moment of inertia of the body was equal to $I_{xx} = 10.92 \cdot 10^{-10}$ kg m$^2$ (cf. [2]). Note that, because of symmetric wing kinematics, inertia of the wings did not affect the time evolution of the roll angle.

# S3 Comparing experimental measurements with theoretical predictions

This supplementary material contains an extended discussion of the diagram shown in figure 6($a$). The diagram consists of a color plot that visualizes the theoretical estimate of $\psi_{rms}$ given by equations (14)-(15), and a set of points that corresponds to data from various experiments and our numerical simulation of a bumblebee. For every point marker, the coordinates $(Tu_w, \theta_{vk})$ are determined using the definition of these two dimensionless numbers, (5) and (4), respectively. The color is determined by $\psi_{rms}$ measured in the corresponding experiment or numerical simulation.

The triangles in figure 6($a$) correspond to the 1-DOF robotic flapper experiments described in section 3. To calculate $Tu_w$, we use the estimate of $W'$ given in supplementary material S4. The markers are filled with color according to the measured values of $\psi_{rms}$, see figure 3($c$). The lower-right point corresponds to the smallest flapping frequency $f = 16.6$ Hz, and upper-left point corresponds to the largest frequency $f = 25.9$ Hz.

The diamond marker visualizes the bumblebee numerical simulation data from section 4. In this case, we evaluate $f_{vk}$ and $W'$ using an auxiliary numerical simulation of the flow past a cylinder with the bee model removed. We thus obtain $f_{vk} = 25$ Hz and $W' = 1.8$ m/s at the position of the insect, yielding $Tu_w = 0.46$ and $\theta_{vk} = 6$.

Circles and squares in figure 6 show the experimental points for hummingbird [6] and hawkmoth [5], respectively, flying in the wakes behind circular cylinders. In the hummingbird experiments [6], the diameter of the cylinder $D$ varied between 2 cm and 9 cm and the inflow velocity $U_\infty$ varied between 3 and 12 m/s. The distance $x$ between the cylinder axis and the feeder was fixed to 15 cm. The distance between the animal's center of mass and the feeder is equal to the wing length, approximately. We therefore use the values of $W'$ at distance $x + R$ from the cylinder axis in our calculations. We evaluated $f_{vk}$ and $W'$ using formulae from supplementary material S4.

The filled circles correspond to the cases when the animals are found able to fly stably. The largest values of $\psi_{rms}$ equal to 29 deg and 23 deg in the theory and in the exper-

iment, respectively, correspond to the test case with the largest cylinder diameter $D$ and the largest velocity $U_\infty$. In the medium cylinder case, however, the theory tends to slightly underestimate the effect of $U_\infty$ compared to the experiment. For the smallest cylinder, $\psi_{rms}$ is of order 2 deg, which is virtually the same as without cylinder treatment.

The white circle corresponds to a flight in the wake of the largest cylinder at 12 m/s. It shows the largest $\psi_{rms}$ on the diagram, in agreement with the experimental observation that the birds were unable to fly and feed stably in that regime.

The squares in the diagram correspond to the hawkmoth experiments [5]. In those experiments, $D$ was equal to 5 cm or 10 cm and $U_\infty$ varied between 0.5 and 2 m/s. The relative distance between the cylinder surface and the feeder varied between 0.5 and 10. Therefore, the relative distance $x/D$ between the cylinder axis and the feeder varied between 1 and 10.5. Since the original data in [5] is reported in terms of the roll amplitude $\Psi$, we use the relationship $\psi_{rms} = \Psi/\sqrt{2}$ of a sine wave signal. All flights fall into the area $\psi_{rms}$ between 3 deg and 21 deg according to the theory and 4 deg and 27 deg, as measured in the experiment.

In addition to the color plot shown in figure 6($a$), it is instructive to view the same data as a function of one variable only. We transform (14)-(15) to obtain

$$\frac{\psi_{rms}}{\theta_{vk}} = \frac{180 \text{ deg}}{\sqrt{2}\pi} \frac{1}{2\pi} \left( \frac{c_{\tau 1}}{\kappa_{fct}} Tu_w + \frac{1}{2} \frac{c_{\tau 2}}{\kappa_{fct}} Tu_w^2 \right). \tag{S1}$$

In figure SF1, we plot the experiment data points $\psi_{rms}/\theta_{vk}$ versus $Tu_w$, and visualize the theoretical relationship (S1). This presentation allows better visual assessment of the agreement between the theory and the experiments. The data points collapse in a single band, in agreement with the theoretical prediction.

The theoretical curve can thus be seen as a nonlinear regression line with two regression coefficients, $c_{\tau 1}/\kappa_{fct}$ and $c_{\tau 2}/\kappa_{fct}$. We suggest the following procedure to evaluate them, yielding the values (22).

- Define the target function as the r.m.s. error between the theoretical and the experimental values of $\psi_{rms}$.
- Find a pair $(c_{\tau 1}/\kappa_{fct}, c_{\tau 2}/\kappa_{fct})$ that minimizes the target function.

Since the data sets in each experiment are too small to determine regression coefficients specific to each flier, we prefer to use all available data points for optimization, and determine a pair of regression coefficients suitable for all fliers considered in this study.

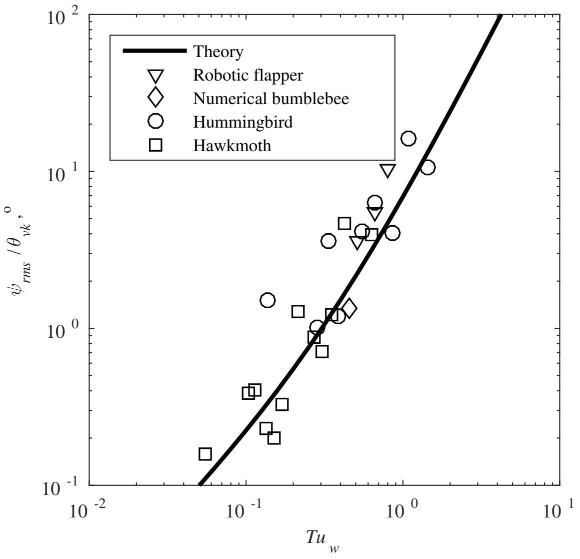


Figure SF1: Comparison between the theoretical functional relation (S1) and the data available from experiments and a numerical simulation. The theoretical estimate assumes $c_{\tau 1}/\kappa_{fct} = 0.267$ and $c_{\tau 2}/\kappa_{fct} = 1.603$.

# S4 Flow unsteadiness in the wake of a cylinder

The equations in section 2 relate the amplitude of the roll angle oscillation $\Psi$ to the unsteady inflow parameters provided in terms of the mean inflow velocity $U_0$ at the position of the flapper, the r.m.s. lateral velocity fluctuation $W'$ and the velocity fluctuation frequency $f_{vk}$. These parameters can quantify different types of time-periodic flows, which makes the theory generally applicable to different biologically relevant unsteady winds. When restricting its scope to flapping flight in the vortex street of a cylinder, it is important to relate $U_0$, $W'$ and $f_{vk}$ to the parameters used in the experiments such as the far-field inflow velocity $U_\infty$, the diameter of the cylinder $D$, and the relative distance from the cylinder to the flapper $x/D$. We provide in this supplementary material some useful empirical relations that fit the data from earlier experimental and numerical studies of the flow past a cylinder. More information about the wakes of circular cylinders can be found in the specialized literature (see [1, 7] and references therein).

Let us define the Reynolds number based on the diameter of the cylinder as $Re_D = U_\infty D/\nu$, and the Strouhal number as $St = f_{vk}D/U_\infty$. We use the relation between $St$ and $Re_D$ based on the data provided in [1],

$$St = 0.2302 - 0.0063 \log_{10} Re_D, \tag{S2}$$

which is valid for a broad range $Re_D = 10^3 ... 10^5$. Thus, knowing $U_\infty$ and $D$, it is straightforward to calculate $f_{vk}$.

Behind the cylinder, there is a velocity deficit. We quantify it by considering the time-averaged streamwise velocity in a streamwise plane that passes through the cylinder axis. We denote it as $U_0$, since this is also the mean inflow velocity for a flapper, if it flies in the wake of the cylinder. At $Re_D$ of about 4000, we refer to [7] which yields

$$\frac{U_0}{U_\infty} = \begin{cases} -0.267(\frac{x}{D} - 0.5), & 0.5 \leq \frac{x}{D} \leq 1.75, \\ 1 - \dfrac{1}{2.529 \ln \frac{x}{D} - 0.665}, & \frac{x}{D} > 1.75. \end{cases} \tag{S3}$$

The r.m.s. lateral velocity fluctuation in the same plane is approximated using the data in [1] as

$$\frac{W'}{U_\infty} = \begin{cases} 0.507(\frac{x}{D} - 0.5), & 0.5 \leq \frac{x}{D} \leq 1.75, \\ 0.8 \cdot 0.8752^{\frac{x}{D}}, & \frac{x}{D} > 1.75. \end{cases} \tag{S4}$$

Comparison between [1] and [7] suggests that the variance of the lateral velocity is not very sensitive to $Re_D$ within the range $Re_D = 10^3 ... 10^5$.

# S5 The effect of roll about the longitudinal body axis

In this supplementary material, let us analyze the situation when the flier only rolls about the longitudinal body axis $Ox_b$, see figure SF2. The body pitch angle $\beta$ is constant. Note that, since only one degree of freedom is unlocked, the roll angle estimates obtained in section 2.1 do not depend on the inclination of the roll axis with respect to the horizontal plane. Therefore, from the point of view of roll amplitude, it is unimportant whether the flapper rolls about the longitudinal body axis or about the mean flow direction. More accurate approximation would require all three body angles vary in time, which would greatly complicate the analysis, probably without adding any conceptually new insights in the dynamics of the system. The analysis in section 2.2, however, does depend on the selected orientation of the roll axis. Let us derive a formula for the vertical force deficit $\Delta \overline{F}_z$ that accounts for non-zero $\beta$.

In a steady and level flight, the only wingbeat-averaged aerodynamic force acting on the body is the vertical force $\overline{F}_{z0}$. Now, in this supplementary material, let $\psi$ denote the angle of rotation about $Ox_b$ (figure SF2$a$). Under the assumption of the aerodynamic force being invariant in the body reference frame $Ox_b y_b z_b$, the aerodynamic force $F(t)$ of a flier rolling in an unsteady flow is constrained to the surface of a cone, as shown in figure SF2($a$). In the body reference frame, the longitudinal component of $F$ does not depend on $\psi$, i.e.,

$$F_{xb} = \overline{F}_{z0} \sin \beta, \tag{S5}$$

but the normal component varies as shown in figure SF2($b$), yielding

$$F_{zb} = \overline{F}_{z0} \cos \beta \sin \psi. \tag{S6}$$

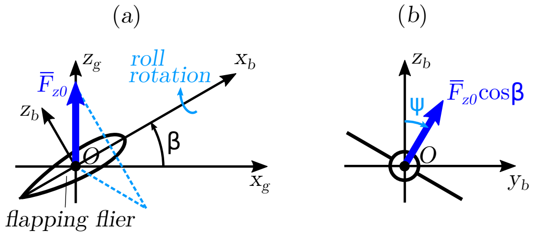


Figure SF2: $(a)$ Schematic drawing of the flier, the aerodynamic force $\overline{F}_{z0}$ acting on it in level flight, its body pitch angle $\beta$, and the direction of roll rotation about the longitudinal body axis $Ox_b$. $(b)$ Direction of the component of the aerodynamic force in a plane normal to $Ox_b$, when the flier rotates at an angle $\psi$ about $Ox_b$.

Therefore, the vertical component of the aerodynamic force in the laboratory reference frame $O_g x_g y_g z_g$ is determined as

$$\begin{aligned} F_{zg} &= F_{zb}\cos\beta + F_{xb}\sin\beta \\ &= \overline{F}_{z0}\cos\psi + \overline{F}_{z0}\sin^2\beta(1-\cos\psi). \end{aligned} \tag{S7}$$

After time averaging, we obtain

$$\overline{F}_{zg} = \overline{F}_{z0} J_0(\Psi) + \overline{F}_{z0}\sin^2\beta(1 - J_0(\Psi)). \tag{S8}$$

Finally, the vertical force deficit is estimated as

$$\Delta\overline{F}_z = \overline{F}_{z0} - \overline{F}_z \approx \overline{F}_{z0}\frac{\Psi^2}{4}\cos^2\beta. \tag{S9}$$

Compared to (19), the only difference is a constant factor $\cos^2\beta$, which is close to 1 for small $\beta$. In more realistic situations when $\beta$ as well as $\psi$ vary over time, or when all three body angles vary, more complex relations can be derived similarly, but they are beyond the scope of this paper.

# References

[1] B. Cantwell and D. Coles. An experimental study of entrainment and transport in the turbulent near wake of a circular cylinder. *Journal of Fluid Mechanics*, 136:321–374, 1983.

[2] T. Engels, D. Kolomenskiy, K. Schneider, F.-O. Lehmann, and J. Sesterhenn. Bumblebee flight in heavy turbulence. *Physical Review Letters*, 116(2):028103, 2016.

[3] T. Engels, D. Kolomenskiy, K. Schneider, and J. Sesterhenn. FluSI: A novel parallel simulation tool for flapping insect flight using a Fourier method with volume penalization. *SIAM Journal on Scientific Computing*, 2015. in press.

[4] I. Kitamura, H. Tanaka, M. Maeda, and H. Liu. Assessing aerodynamic performance of hummingbird-inspired flapping system. In *Proceedings of Annual Meeting, Bioengineering Division, JSME*, page 2B21, 2015.

[5] V. M. Ortega-Jimenez, J. S. M. Greeter, R. Mittal, and T. L. Hedrick. Hawkmoth flight stability in turbulent vortex streets. *Journal of Experimental Biology*, 216(24):4567–79, 2013.

[6] V. M. Ortega-Jimenez, N. Sapir, M. Wolf, E. A. Variano, and R. Dudley. Into turbulent air: size-dependent effects of von Kármán vortex streets on hummingbird flight kinematics and energetics. *Proceedings. Biological sciences / The Royal Society*, 281(1783):20140180, 2014.

[7] P. Parnaudeau, J. Carlier, D. Heitz, and E. Lamballais. Experimental and numerical studies of the flow over a circular cylinder at Reynolds number 3900. *Physics of Fluids*, 20(8):085101, 2008.

[8] K. Suga, H. Tanaka, and H. Liu. Investigation of passive motions and aerodynamics of a hummingbird-inspired flapping wing. In *Proceedings of JSME Annual Meeting*, page J0220403, 2014.

[9] H. Tanaka, H. Suzuki, I. Kitamura, M. Maeda, and H. Liu. Lift generation of hummingbird wing models with flexible loosened membranes. In *2013 IEEE/RSJ International Conference on Intelligent Robots and Systems*, pages 3777–3783, 2013.
